# Supplementary material for: Ion neutralisation mass-spectrometry route to radium monofluoride (RaF)
Source: arXiv:1310.1511 ancillary file (2013-11-21)
Supplement: Supplementary file 1 [file Suppl-6r.pdf]

# Supplementary material for the article ''Ion neutralisation mass-spectrometry route to radium monofluoride (RaF)"

T.A. Isaev,[1] S. Hoekstra,[2] L. Willmann,[2] and R. Berger[1,*]

[1] *Clemens-Schöpf Institute, TU Darmstadt, Petersenstr. 22, 64287 Darmstadt, Germany*

[2] *Kernfysisch Versneller Instituut, University of Groningen, Zernikelaan 25, 9747 AA Groningen, The Netherlands*

## BASIS SETS AND NUCLEAR MODEL

Both basis sets and nuclear model for four-component (4c) calculations with the DIRAC program package [1] are the same as in http://arxiv.org/abs/1302.5682 (see supplementary material there). For calculations with the program package Molpro [2, 3], the relativistic effective core potential (RECP) ECP78MDF together with the corresponding basis set on radium were employed whereas the all electron basis set def2-QZVP was used for fluorine. For two-component ZORA calculations with a modified version of Turbomole [4], the even-tempered basis set from http://arxiv.org/abs/1206.6013 was used.

## DISSOCIATION ENERGY CALCULATION

The dissociation energy of $RaF^+$ was computed in the following way: we calculated by RCC-SD (with a large active space extending to orbitals with an energy of up to 1000 Hartree) the total energy for $RaF^+$ (−25132.5313 Hartree) at the equilibrium distance and the ionisation energy for RaF (both adiabatic and vertical are close) of $I_{\mathrm{adiabatic}} = 4.96$ eV. Additionally, we calculated the energies of closed-shell $Ra^{2+}$ and $F^-$ separately: $E(\mathrm{Ra}^{2+}) = -25032.2550$ Hartree and $E(\mathrm{F}^-) = -99.8226$ Hartree. We combined the resulting energies with the experimental ionisation energies $I$ for Ra and its ions, namely $I(\mathrm{I}) = 5.28$ eV [5] and $I(\mathrm{II}) = 10.15$ eV [6], and the electron affinity $A$ for F, namely $A = 3.40$ eV [7], to obtain an estimate for the dissociation energy of $RaF^+$ (see Table) on the three step route $\mathrm{RaF}^+ \longrightarrow \mathrm{Ra}^{2+}+\mathrm{F}^-$; $\mathrm{Ra}^{2+} + \mathrm{e}^- \rightarrow \mathrm{Ra}^+$; $\mathrm{F}^- \rightarrow \mathrm{F} + \mathrm{e}^-$, which we consider more reliable than the one step route of an estimate via $\mathrm{RaF}^+ \longrightarrow \mathrm{Ra}^++\mathrm{F}$. From the former we also obtained the dissociation energy of RaF, when combined with the computed ionisation energy of RaF and the experimental first ionisation energy of Ra. The notation RaF→ Ra + F (one step) in the table means, instead, that the dissociation energy was obtained just by separate calculations of the energies of RaF, Ra and F. We performed similar calculations for neutral barium monofluoride, either via the three step route using the experimental ionisation energies of Ba and its ions, namely $I(\mathrm{I}) = 5.21$ eV [8] and $I(\mathrm{II}) = 10.00$ eV [9], or the one step route.

In the table, the program package is given in parentheses together with the method used for calculation. E.g. (MOLPRO rccsd(t) + 10e AREP ) means that the rccsd(t) module of the Molpro package was used in combination with the scalar-relativistic (spin-averaged) 10-electron Stuttgart Energy-Consistent (EC) relativistic effective core potential on Ra. The equilibrium distance $R_\mathrm{e}$ and harmonic vibrational wavenumber $\tilde{\omega}_\mathrm{e}$ were obtained from a fit of the raw data to a Morse potential.

Electronic ground $^1\Sigma_0$ state of $RaF^+$

| Method (Code + details) | Dissociation energy in eV ($10^4$ cm$^{-1}$) | Molecular parameters $R_\mathrm{e}/a_0$, $\tilde{\omega}_\mathrm{e}/(\mathrm{cm}^{-1})$ |
|---|---|---|
| 4c RCC-SD | | |
| (DIRAC, AS 1000 Hartree) | | |
| $\mathrm{RaF}^+ \rightarrow \mathrm{Ra}^+$+F (three step) | 5.59 (4.51) | 4.14, 502 |

Electronic ground $^2\Sigma_{1/2}$ state of RaF

| Method (Code + details) Route | Dissociation energy in eV ($10^4$ cm$^{-1}$) | Ionisation energy in eV ($10^4$ cm$^{-1}$) | Molecular parameters $R_e/a_0$, $\tilde{\omega}_e$/cm$^{-1}$ |
|---|---|---|---|
| 4c RCC-SD (DIRAC, AS 1000 Hartree) RaF → Ra + F (three step) | 5.28 (4.26) | 4.96 (4.00) | $4.29^a$, $431^a$ |
| 4c RCC-SD (DIRAC, AS 10 Hartree) RaF → Ra + $F^c$ | $3.98^b$ (3.21) | | $4.24^b$, $428^b$ |
| 1c RCC-SD(T) (MOLPRO, rccsd(t) + 10e AREP) RaF → Ra + F (three step) | 5.37 (4.33) | 4.96 | |
| 1c RCC-SD(T) (MOLPRO, rccsd(t) + 10e AREP) RaF → Ra + F (one step) | 5.22 (4.21) | | 4.30, 417 |
| 2c ZORA/GHF (tm2c) RaF → Ra + F (one step) | 4.07 (3.28) | | |
| 2c ZORA/DFT (tm2c, B3LYP) RaF → Ra + F (three step) | 6.24 (5.03) | 5.12 (4.13) | |
| 2c ZORA/DFT (tm2c, B3LYP) RaF → Ra + F (one step) | 5.52 (4.45) | | |

a) Ref. [10] b) Ref. [11], c) see Ref. [11] for procedure of this estimate

Electronic ground $^2\Sigma_{1/2}$ state of BaF

| Method (Code + details) Route | Dissociation energy in eV ($10^4$ cm$^{-1}$) | Molecular parameters $R_e/a_0$, $\tilde{\omega}_e$/cm$^{-1}$ |
|---|---|---|
| Experiment | $5.80\pm0.09^a$ | $4.09^a$, $469^a$ |
| 4c RCC-SD (DIRAC, AS 1000 Hartree) BaF → Ba + F (three step) | 5.79 (4.67) | $4.15^b$, $456^b$ |
| 1c RCC-SD(T) (MOLPRO, rccsd(t) + 10e AREP) BaF → Ba + F (three step) | 5.88 (4.74) | |
| 1c RCC-SD(T) (MOLPRO, rccsd(t) + 10e AREP) BaF → Ba + F (one step) | 5.58 (4.50) | 4.16, 459 |
| 1c RCC-SD(T) (MOLPRO, rccsd(t) non-rel) BaF → Ba + F (one step) | 6.06 (4.89) | |

a) Ref. [12], b) Ref. [10]

## POTENTIAL ENERGY VALUES OF ENERGETICALLY LOW-LYING ELECTRONIC STATES OF RAF$^+$ AND RAF

Data for the cationic ground state are from this work, data for the various neutrals states are from Ref. [10].

```
Raw data (in Mathematica format) of the FS-CCSD energy (in Hartree) at
different internuclear distances (in units of the Bohr radius).
All energies are shifted by -25130.0 Hartree.
Ground state \Sigma_0 of RaF+:
{{3.4, -2.453368753573159}, {3.7, -2.5093798}, {3.9, -2.5255991},
{4.0, -2.52941637281}, {4.1, -2.5310378336}, {4.2, -2.53086613},
{4.25, -2.5302159713683}, {4.3, -2.52924}, {4.4, -2.526443947},
{4.5, -2.52271512512}, {4.7, -2.51321679821}, {5.0, -2.49593046755399},
{5.5, -2.464539528493333}}
Ground \Sigma_1/2 state of RaF:
{{3.4, -2.61896827} , {3.7, -2.6810475693}, {3.9, -2.701438115},
{4.0, -2.707355929}, {4.1, -2.71107952}, {4.15, -2.712245222046},
{4.2, -2.7130062}, {4.25, -2.7134023758}, {4.3, -2.7134702786},
{4.4, -2.71275215884}, {4.5, -2.711086221825} , {4.7, -2.7056587},
{5.0, -2.694317976377}, {5.5, -2.672360131139}}
First excited (\Pi_1/2) of RaF:
{{3.4, -2.55914478}, {3.7, -2.620627218741}, {3.9, -2.64091361},
{4.0, -2.646828821}, {4.1, -2.650570973}, {4.15, -2.651751778991},
4.2, -2.65253083}, {4.25, -2.65294745}, {4.3,-2.653037666863},
{4.4, -2.6523680724}, {4.5, -2.650753595208}, {4.7, -2.6454302},
{5.0, -2.634233283523}, {5.5, -2.612462214729}}
2nd excited (\Pi_3/2+\Delta_3/2) of RaF:
{{3.4, -2.551178387668}, {3.7, -2.61206742}, {3.9, -2.63216039},
{4.0, -2.63814297}, {4.1, -2.64206593}, {4.15, -2.643361819482},
{4.2, -2.64426494}, {4.25, -2.64481137}, {4.3, -2.64503509},
{4.4, -2.64463889}, {4.5, -2.643301941935}, {4.7, -2.6385357},
{5.0, -2.628161427147}, {5.5, -2.607683096769}}
3rd excited (\Pi_3/2+\Delta_3/2) of RaF:
{{3.4, -2.547995013745}, {3.7, -2.61050150}, {3.9, -2.63125097},
{4.0, -2.63724423}, {4.1, -2.64096208}, {4.15, -2.642110746598},
{4.2, -2.64285196}, {4.25, -2.64322834}, {4.3, -2.64327798},
{4.4, -2.64253077}, {4.5, -2.640847235558}, {4.7, -2.635417596957},
{5.0, -2.624139970427}, {5.5, -2.602951138640}}
4th excited (\Delta_5/2) of RaF:
{{3.4, -2.545390225903}, {3.7, -2.60766727}, {3.9, -2.62839117},
{4.0, -2.63450950}, {4.1, -2.63844850}, {4.15, -2.639726110290},
{4.2, -2.64060121}, {4.25, -2.64111330}, {4.3, -2.64129857},
{4.4,-2.64081834}, {4.5, -2.639392742032}, {4.7, -2.634446697961},
{5.0, -2.623813022317}, {5.5, -2.602403068209}}
5th excited (\Sigma_1/2 state) of RaF:
{{3.4, -2.538839380264}, {3.7, -2.60209643}, {3.9, -2.62351221},
{4.0, -2.62994016}, {4.1, -2.63415707}, {4.15, -2.635561158826},
{4.2, -2.63655436}, {4.25, -2.63717627}, {4.3, -2.63746324},
{4.4, -2.63716298}, {4.5, -2.635888067583}, {4.7, -2.631166233721},
{5.0, -2.620716634014}, {5.5, -2.599905982435}}
```

* robert.berger@tu-darmstadt.de

[1] DIRAC, a relativistic ab initio electronic structure program, Release DIRAC11 (2011), written by R. Bast, H. J. Aa. Jensen, T. Saue, and L. Visscher, with contributions from V. Bakken, K. G. Dyall, S. Dubillard, U. Ekström, E. Eliav, T. Enevold-

sen, T. Fleig, O. Fossgaard, A. S. P. Gomes, T. Helgaker, J. K. Lærdahl, J. Henriksson, M. Iliaš, Ch. R. Jacob, S. Knecht, C. V. Larsen, H. S. Nataraj, P. Norman, G. Olejniczak, J. Olsen, J. K. Pedersen, M. Pernpointner, K. Ruud, P. Sałek, B. Schimmelpfennig, J. Sikkema, A. J. Thorvaldsen, J. Thyssen, J. van Stralen, S. Villaume, O. Visser, T. Winther, and S. Yamamoto (see http://dirac.chem.vu.nl).

[2] H.-J. Werner, P. J. Knowles, G. Knizia, F. R. Manby, and M. Schütz, WIREs Comput. Mol. Sci. **2**, 242 (2012).

[3] MOLPRO, version 2012.1, a package of *ab initio* programs, H.-J. Werner, P. J. Knowles, G. Knizia, F. R. Manby, M. Schütz, P. Celani, T. Korona, R. Lindh, A. Mitrushenkov, G. Rauhut, K. R. Shamasundar, T. B. Adler, R. D. Amos, A. Bernhardsson, A. Berning, D. L. Cooper, M. J. O. Deegan, A. J. Dobbyn, F. Eckert, E. Goll, C. Hampel, A. Hesselmann, G. Hetzer, T. Hrenar, G. Jansen, C. Köppl, Y. Liu, A. W. Lloyd, R. A. Mata, A. J. May, S. J. McNicholas, W. Meyer, M. E. Mura, A. Nicklass, D. P. O'Neill, P. Palmieri, D. Peng, K. Pflüger, R. Pitzer, M. Reiher, T. Shiozaki, H. Stoll, A. J. Stone, R. Tarroni, T. Thorsteinsson, and M. Wang, see http://www.molpro.net.

[4] R. Ahlrichs, M. Bär, M. Häser, H. Horn, and C. Kölmel, Chem. Phys. Lett. **162**, 165 (1989).

[5] J. A. Armstrong, J. J. Wynne, and F. S. Tomkins, J. Phys. B: Atom. Molec. Phys. **13**, L133 (1980).

[6] E. Rasmussen, Z. Phys. **86**, 24 (1933).

[7] C. Blondel, C. Delsart, and F. Goldfarb, J. Phys. B: Atom. Mol. Opt. Phys. **34**, L281 (2001).

[8] B. H. Post, W. Vassen, W. Hogervorst, M. Aymar, and O. Robaux, Journal of Physics B **18**, 187 (1985).

[9] H. Karlsson and U. Litzen, Physica Scripta **60**, 321 (1999).

[10] T. A. Isaev and R. Berger, ArXiv e-prints (2013), arXiv:1302.5682 [physics.chem-ph].

[11] T. A. Isaev, S. Hoekstra, and R. Berger, Phys. Rev. A **82**, 052521 (2010).

[12] G. Blue, J. Margrave, T. Ehlert, and J. Green, Nature **199**, 804 (1963).
